# Supplementary material for: EndoVLM: An Endoscopy Vision-Language Pre-training Model via Anatomy-Guided Sparsity and Progressive Alignment
Source: arXiv:2608.04472 source file (2026-08-05)
Supplement: Supplementary file 1 [file appendix.tex]

% Appendix intentionally left empty for the arXiv preprint.
